# Supplementary material for: CAE-Bench: Benchmarking AI Agents for Reusable CAE Solver Development
Source: arXiv:2611.21273 source file (2026-11-26)
Supplement: Supplementary file 2 [file cavity_reference_checks.tex]

\begin{table}[!htbp]
\centering
\small
\begin{tabularx}{\linewidth}{@{}Xrrr@{}}
\toprule
Recorded comparison & \(u\) NRMSE & \(v\) NRMSE & \(p\) NRMSE \\
\midrule
Spatial refinement, L1--L2 & \(1.859\times10^{-3}\) & \(2.596\times10^{-3}\) & \(8.688\times10^{-3}\) \\
Halved time step & \(9.846\times10^{-5}\) & \(1.434\times10^{-4}\) & \(2.024\times10^{-5}\) \\
OpenFOAM, N64 & \(2.226\times10^{-3}\) & \(3.790\times10^{-3}\) & \(7.345\times10^{-3}\) \\
OpenFOAM, N128 & \(2.688\times10^{-3}\) & \(4.267\times10^{-3}\) & \(5.994\times10^{-3}\) \\
\bottomrule
\end{tabularx}
\caption{Recorded consistency checks for each field of the RC7 fixed-cavity reference results (\texttt{cc-lid-driven-cavity}). The hash of the selected reference results matches the historical certificate. These NRMSE values are not newly computed RMS case scores.}
\label{tab:cavity-reference-checks}
\end{table}
